# Supplementary material for: Distillation-Enhanced Physical Adversarial Attacks
Source: arXiv:2501.02232 source file (2025-01-04)
Supplement: Supplementary file 1 [file 6_appendix.tex]

\appendix
In the supplementary materials, we present additional experimental results from both digital and physical domains to confirm the effectiveness of the proposed method. We also analyze the pattern similarity of adversarial patches, explaining why optimized patches perform poorly in constrained color spaces and highlighting the factors that contribute to the superior performance of the proposed methods.

\subsection{Visualized Digital Experiments}
Here, we conduct digital experiments on the INRIA test set using four models: YOLOv2, YOLOv3, YOLOv5, and FasterRCNN. The experiments are performed in a white-box setting, where the same models are used for both generating adversarial patches and testing, with the attack targeting the `person' category. As shown in Fig.~\ref{fig:digital experiment}, the visual results indicate that the adversarial patches generated by the distillation-based method achieve superior attack performance across various models, effectively causing the detectors to miss the ``person" category.

\subsection{Physical Experiment Results}
We conducted physical experiments in some other scenarios in this section, including indoor and outdoor environments. First, we captured images from various scenes and utilized a primary color extractor to identify the dominant colors of the environment, thereby defining the optimization space for stealthy colors. Next, based on our knowledge distillation framework for adversarial patch generation, we used unconstrained-color patches as teacher patches to guide the optimization of student patches (i.e., stealthy patches) within a constrained color space. Finally, we printed the optimized patches and conducted physical experiments in the corresponding scenarios.

As shown in Fig.~\ref{pic:physical experiment}, the four adversarial patches on the left correspond to different physical scenarios with varying dominant colors. These adversarial patches align with the dominant colors of their environments, allowing them to blend seamlessly into the surroundings. Unlike unconstrained-color adversarial patches, which are often vibrant and easily noticeable by the human eye, our method demonstrates superior environmental concealment. Additionally, we quantified the effectiveness of adversarial patches by calculating the Attack Success Rate (ASR) across different scenarios. The ASR is defined as the proportion of successfully attacked frames relative to the total number of frames in a detection video. The results demonstrate that adversarial patches generated using our method achieved an ASR of approximately 90\% across all four scenarios, even when printed on paper and occupying a relatively small area. This highlights the robust attack performance of our method, even under physically constrained conditions.

\subsection{Similarity Analysis of Adversarial Patches}

\begin{figure}[t] 
    \centering 
    \includegraphics[width=\columnwidth]{images/append/append_physical_v1.png}
    \caption{The attack performance and Attack Success Rate (ASR) of the optimized adversarial patches in different scenarios with the YOLOv5s model.}
    \label{pic:physical experiment}
\end{figure}

In our experiments, we observed that although the color spaces used for teacher and student patch optimization differ, their patterns remain similar. Therefore, we quantitatively analyzed the similarities between teacher patches and student patches generated by both non-distillation and distillation methods here, for exploring the factors that enhance attack performance.

\begin{figure*}[t] % 使用 figure* 环境
    \centering
    \includegraphics[width=0.95\textwidth]{images/append/digital_v5_zip.png} % 图片宽度设置为两栏宽度
    \caption{The detection results of different models on the INRIA test set with adversarial patches. The first row of each model presents the adversarial patches generated by the non-distillation method and their detection results, while the second row shows the corresponding results for the distillation method. Clearly, adversarial patches generated within the distillation framework exhibit stronger attack capabilities, effectively deceiving the detector and preventing it from recognizing the ``person" class.}
    \label{fig:digital experiment}
\end{figure*}

The Structural Similarity Index (SSIM) is a widely used image quality assessment metric that evaluates the perceptual quality of images by considering changes in structural information, luminance, and texture. SSIM is designed to model the human visual system's sensitivity to structural variations, providing a more reliable representation of perceived image quality. We use this metric to quantitatively assess the similarity between distilled adversarial patches and teacher patches, and compare it with the non-distillation method. The formula for calculating SSIM is as follows:
\begin{equation}
\mathrm{SSIM}(x,y)=\frac{(2\mu_x\mu_y+C_1)(2\sigma_{xy}+C_2)}{(\mu_x^2+\mu_y^2+C_1)(\sigma_x^2+\sigma_y^2+C_2)}
\end{equation}
where \( \mu_x \) and \( \mu_y \) represent the mean luminance of images \( x \) and \( y \), respectively. \( \sigma_x \) and \( \sigma_y \) denote the standard deviations of images \( x \) and \( y \), respectively. \( \sigma_{xy} \) is the covariance between images \( x \) and \( y \). \( C_1 \) and \( C_2 \) are constants used to avoid division by zero. Typically, \( C_1 = (K_1 L)^2 \) and \( C_2 = (K_2 L)^2 \), where \( K_1 = 0.01 \), \( K_2 = 0.03 \), and \( L \) is the dynamic range (for example, \( L = 255 \) in 8-bit images).

\begin{figure}[tb] 
    \centering 
    \includegraphics[width=\columnwidth]{images/append/similar_v2.png}
    \caption{Adversarial patches with different attack methods under different models.}
    \label{pic:TS_patch}
\end{figure}
As shown in Fig.~\ref{pic:TS_patch}, we compared the adversarial patch patterns optimized by different attack methods across different detection models. For each model, the adversarial patches are presented from left to right as follows: the patch obtained by the non-distillation method, the color-unrestricted patch obtained by the AdvPatch method, and the adversarial patch obtained by our distillation method that AdvPatch serves as the teacher patch. Visually, the adversarial patches obtained by our method are more similar to the teacher patch. 

As shown in Fig.~\ref{pic:TS_patch}, we present the adversarial patch patterns optimized by different methods across four detection models. For each model, the adversarial patches are displayed from left to right as follows: the non-distillation patch, the AdvPatch-generated patch, and the patch from our distillation method. In our method, the adversarial patch from the AdvPatch method serves as the teacher patch, guiding the optimization of the stealthy patch. Visually, we observe that the adversarial patches generated by our method are more similar to the teacher patch.

Meanwhile, we used the SSIM metric to quantitatively evaluate the structural similarity between the adversarial patches generated by the non-distillation method and our distillation method, and the color-unrestricted patch generated by AdvPatch. As shown in Table~\ref{tab:SSIM}, across four models, the SSIM values between the adversarial patches generated by our distillation method and the color-unrestricted patch are higher than those obtained by the non-distillation method, indicating greater consistency, which aligns with our subjective evaluation.

\begin{table}[t]
\caption{The SSIM Similarity Between Adversarial Patches Generated by Different Methods and the Color-Unrestricted Patches}
\resizebox{1.0\columnwidth}{!}{

\centering
\begin{tabular}{c|c|c|c|c}
\hline
Method               & YOLOv2  & YOLOv3 &YOLOv5 &FasterRCNN \\ \hline
non-Distillation           & 0.1020 &  0.0888  & 0.1593& 0.1211 \\ \hline
Ours(Distillation)                       & 0.1044 &  0.0953   & 0.1672& 0.1501\\ \hline
\end{tabular}
\label{tab:SSIM}
}
\end{table}

Both visualizations and SSIM metrics demonstrate that our distillation method effectively improves the similarity between the generated adversarial patches and the color-unrestricted teacher patches. It is clear that more similar patterns lead to better attack performance. This suggests that the unrestricted color space is more conducive to finding the optimal solution for adversarial patches, while the constrained color space may lead to local optima. Additionally, it highlights the effectiveness of our distillation method, which helps adversarial patches escape local optima in the constrained color space, thereby achieving better attack results.
